# Supplementary material for: SpinBench: Perspective and Rotation as a Lens on Spatial Reasoning in VLMs
Source: arXiv:2509.25390 source file (2026-02-28)
Supplement: Supplementary file 1 [file appendix_more_example.pdf]

Task group: identity matching (car)

Task: car\_identity

Question:

<image>  
<image>  
<image>

Two of these images show the same car from different angles. Which one shows a different car?  
Only answer with the capital letter from (A, B, C).

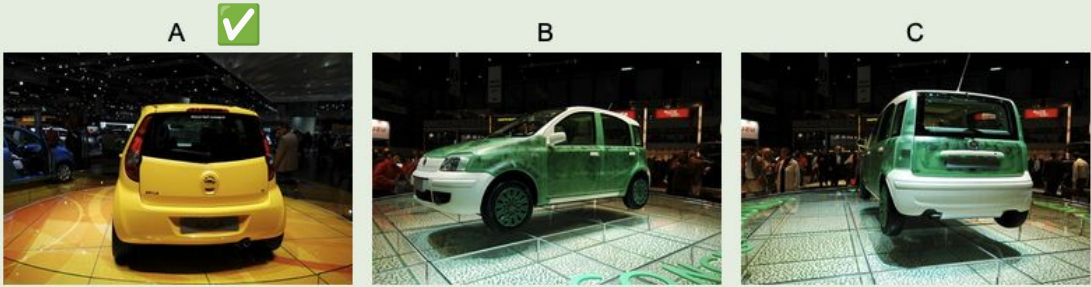

Task: car\_identity\_quartet\_imagefirst

Question:

<image>  
<image>  
<image>  
<image>

Which of these four images (A, B, C, D) shows a different car from the other three?  
Only answer with the capital letter from (A, B, C, D).

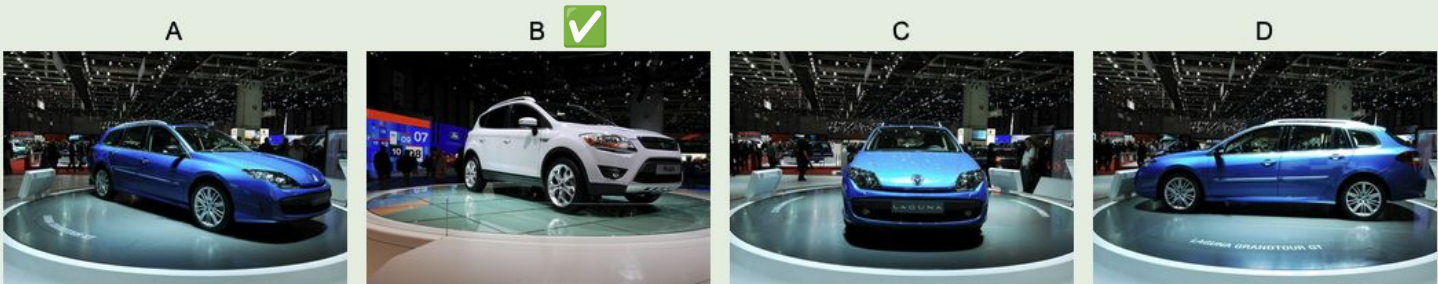

Task: car\_identity\_quartet\_interleaved

Question:

Look at the following four cars:

A. <image>  
B. <image>  
C. <image>  
D. <image>

Which image shows a different car?  
Only answer with the capital letter from (A, B, C, D).

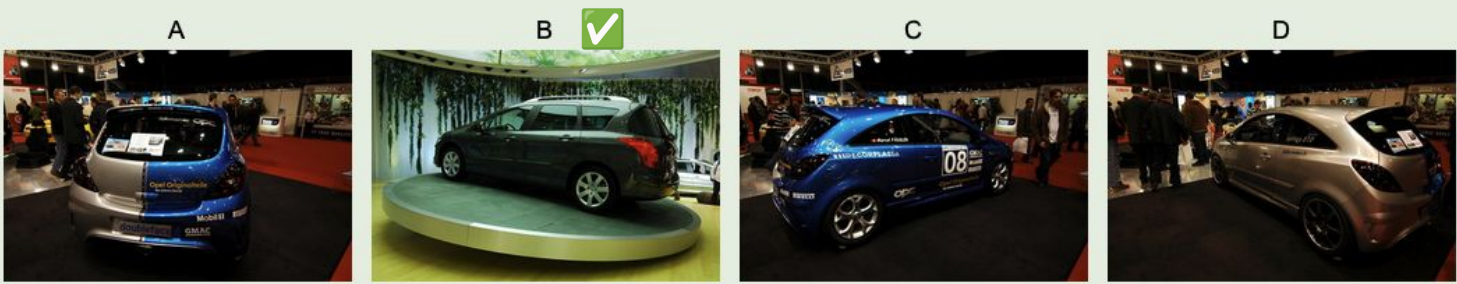

Task: car\_identity\_quartet\_textfirst

Question:

Which of these four images shows a different car from the other three?

A. <image>  
B. <image>  
C. <image>  
D. <image>

Only answer with the capital letter from (A, B, C, D).

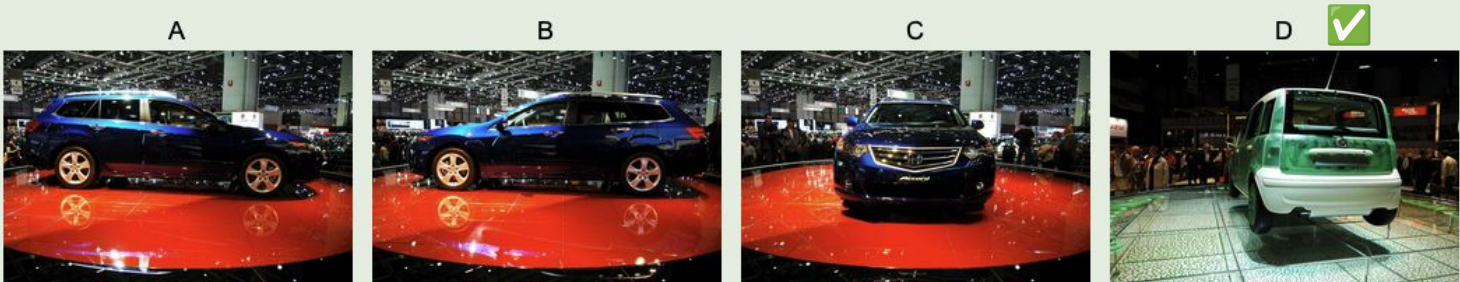



Task group: identity matching (face)

Task: face\_identity

Question:

<image>  
<image>  
<image>  
Two of these images show the same person from different angles. Which one shows a different person?  
Only answer with the capital letter from (A, B, C).

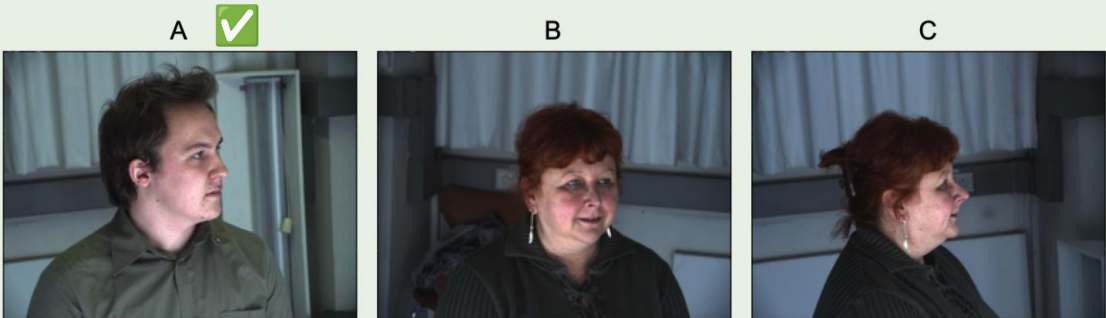

Task: face\_identity\_quartet\_imagefirst

Question:

<image>  
<image>  
<image>  
<image>  
Three photos show the same person, one shows someone different. Which is different?  
Only answer with the capital letter from (A, B, C, D).

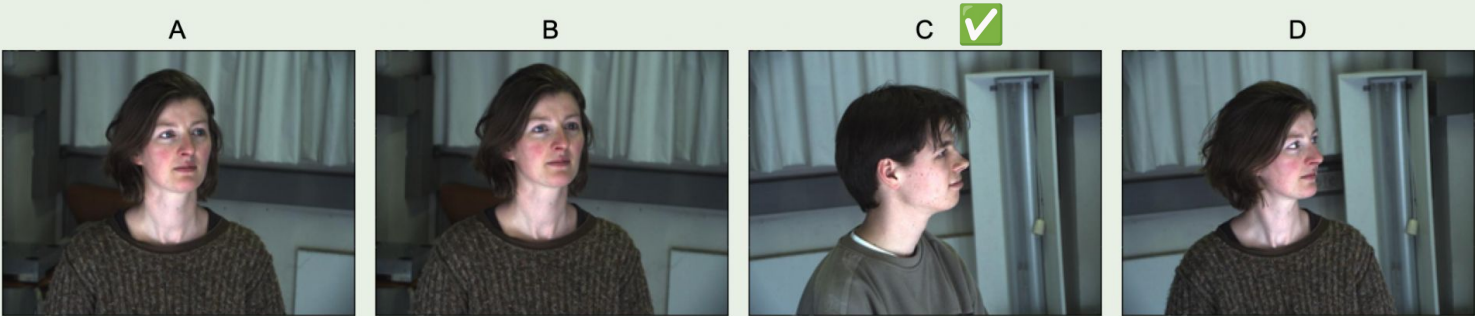

Task: face\_identity\_quartet\_interleaved

Question:

Compare these individuals:  
A. <image>  
B. <image>  
C. <image>  
D. <image>  
Which is the different person?  
Only answer with the capital letter from (A, B, C, D).

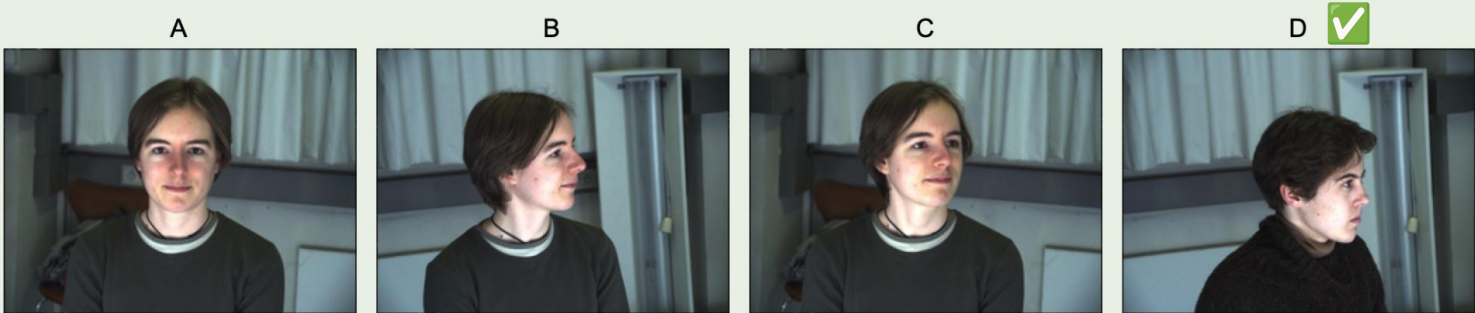

Task: face\_identity\_quartet\_textfirst

Question:

In these four images, three show the same person from different poses, but one shows a different person. Identify the different one.  
A. <image>  
B. <image>  
C. <image>  
D. <image>  
Only answer with the capital letter from (A, B, C, D).

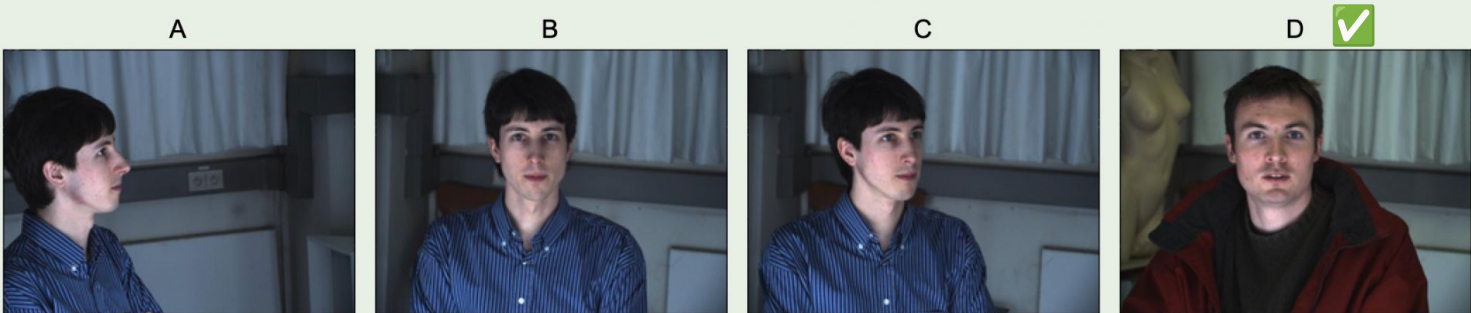

Task group: identity matching (object)

Task: object\_identity\_quartet\_imagefirst

Question:

<image>  
<image>  
<image>  
<image>

Three of these images show the same object at different views. Which one shows the different object?  
Only answer with the capital letter from (A, B, C, D).

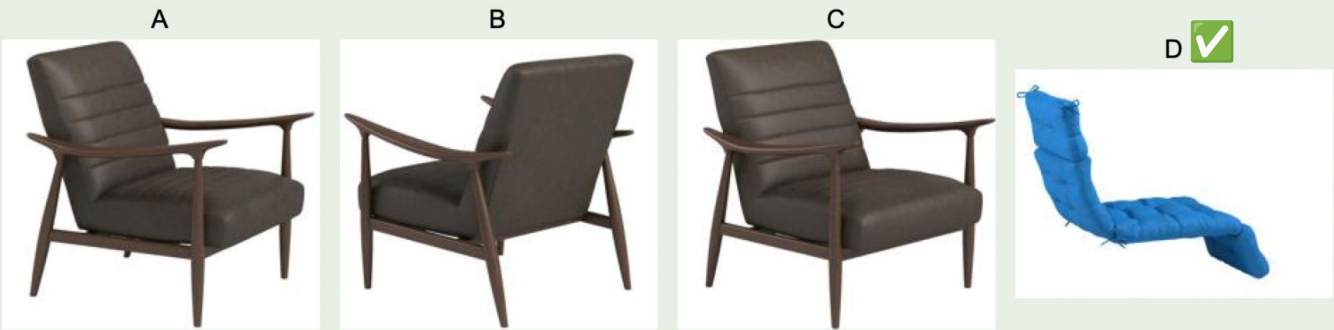

Task: object\_identity\_quartet\_interleaved

Question:

Look at the following four images:

A. <image>  
B. <image>  
C. <image>  
D. <image>

Which image shows a different object?  
Only answer with the capital letter from (A, B, C, D).

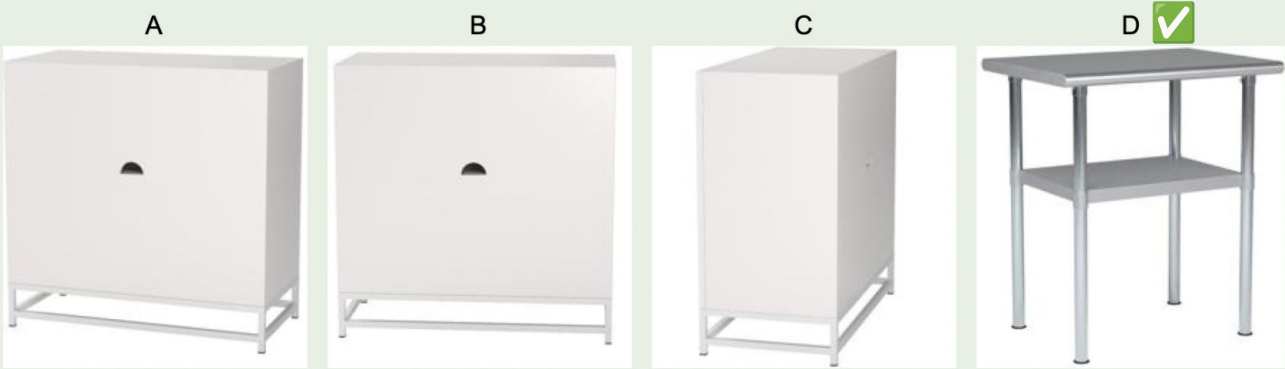

Task: object\_identity\_quartet\_textfirst

Question:

Which of these four images shows a different object from the other three?

A. <image>  
B. <image>  
C. <image>  
D. <image>

Only answer with the capital letter from (A, B, C, D).

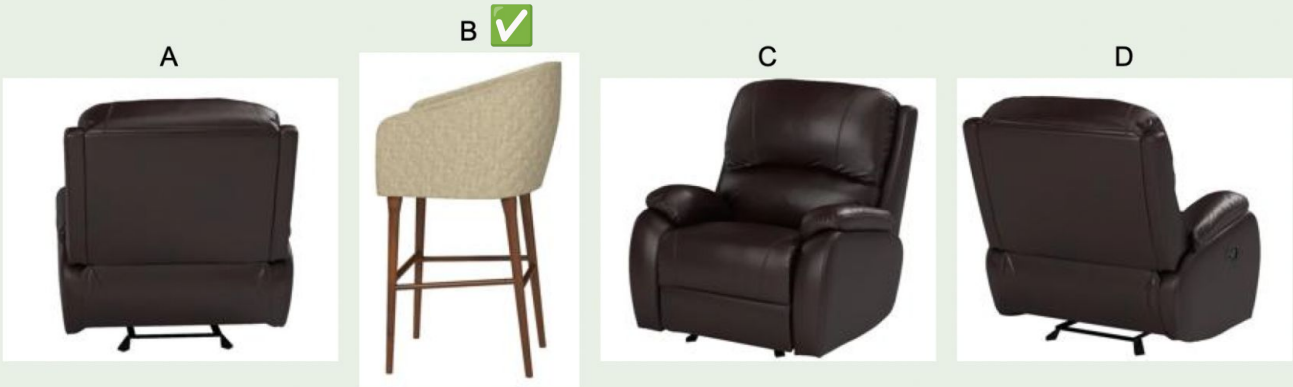

Task group: identity matching (object)

Task: object\_identity\_imagefirst

Question:

<image>  
<image>  
<image>

Which of these three images (A, B, C) shows a different object from the other two?  
Only answer with the captial letter from (A, B, C).

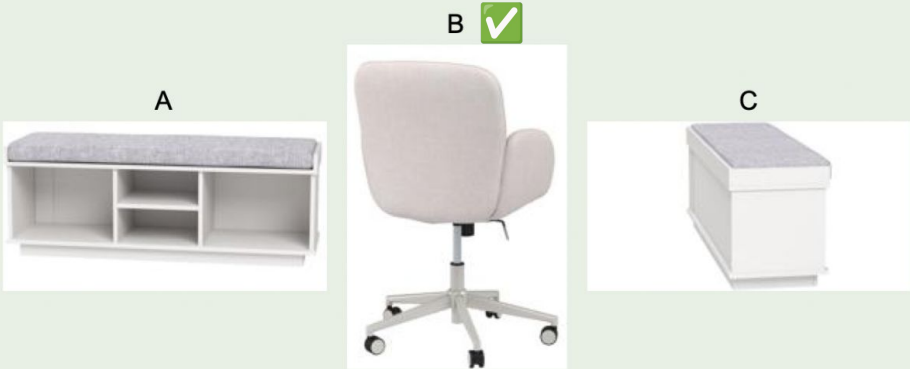

Task: object\_identity\_interleaved

Question:

Look at the following three images:

A. <image>  
B. <image>  
C. <image>

Which image shows a different object?  
Only answer with the captial letter from (A, B, C).

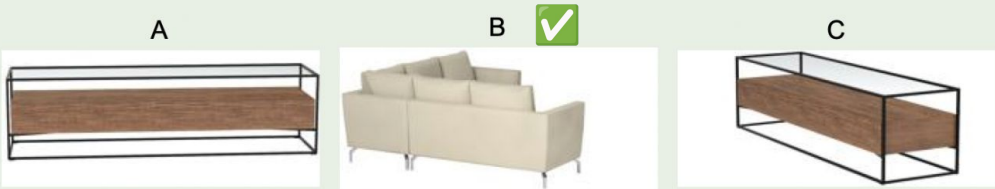

Task: object\_identity\_textfirst

Question:

In those three images, two of them show the same object at different views, but the other one show a different object. Identify which show the different object.

A. <image>  
B. <image>  
C. <image>

Only answer with the captial letter from (A, B, C).

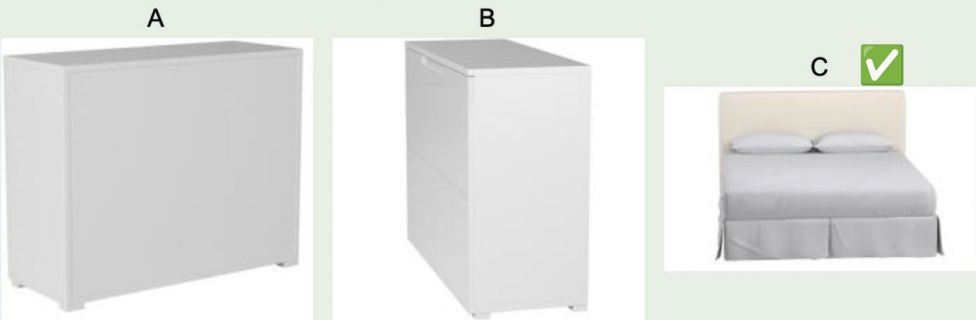



Task group: dynamic rotation (car)

Task: car\_rotation\_classification

Question:

<image>  
<image>

The car rotated from the front view to the second view. Was the rotation clockwise or counterclockwise? A. clockwise, B. counterclockwise  
Only answer with the capital letter from (A, B).  
The camera is stationary and the car rotates in place from the front view.  
Clockwise and counterclockwise are defined from a top-down view.

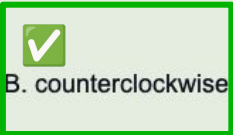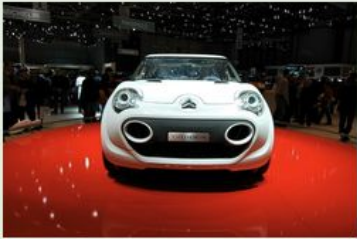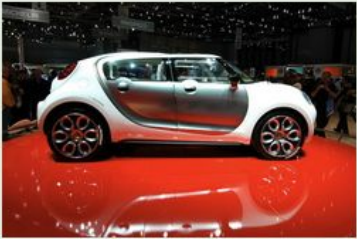

Task: car\_rotation\_classification

Question:

<image>  
<image>

The first image shows the car from the front. In which direction did the car rotate to reach the second view? A. clockwise, B. counterclockwise  
Only answer with the capital letter from (A, B).  
The camera is stationary and the car rotates in place from the front view.  
Clockwise and counterclockwise are defined from a top-down view.

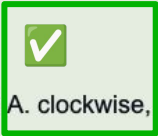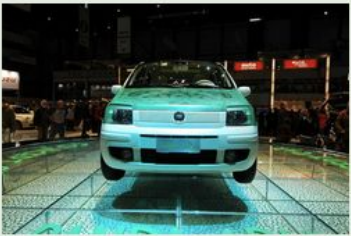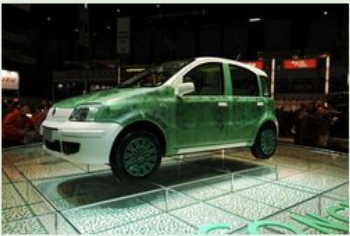

Task group: dynamic rotation (face)

Task: face\_rotation\_classification\_own\_perspective

Question:

<image>  
<image>  
From the person's own perspective, which way did they turn their head? A. right, B. left  
Only answer with the capital letter from (A, B).  
Consider the direction from the person's own perspective (their left vs their right).

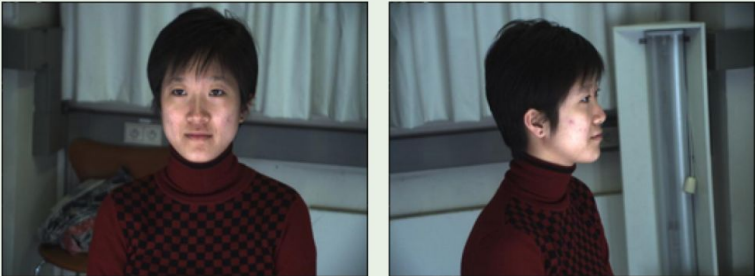

Task: face\_rotation\_classification\_own\_perspective

Question:

<image>  
<image>  
From the person's own perspective, which way did they turn their head? A. right, B. left  
Only answer with the capital letter from (A, B).  
Consider the direction from the person's own perspective (their left vs their right).

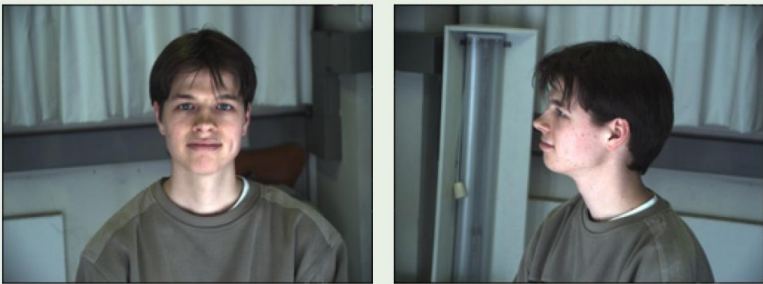

Task: face\_rotation\_classification\_viewer\_perspective

Question:

<image>  
<image>  
From the viewer's perspective, which direction did the person's head turn? A. left, B. right  
Only answer with the capital letter from (A, B).  
Consider the direction from viewer's perspective (viewer's left vs viewer's right).

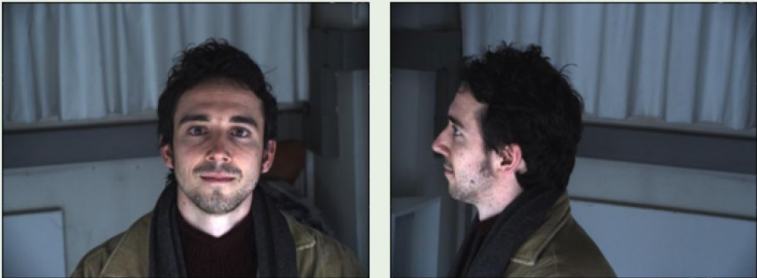

Task: face\_rotation\_classification\_viewer\_perspective

Question:

<image>  
<image>  
Looking at the person from the camera's position, they turned to the A. left, B. right  
Only answer with the capital letter from (A, B).  
Consider the direction from viewer's perspective (viewer's left vs viewer's right).

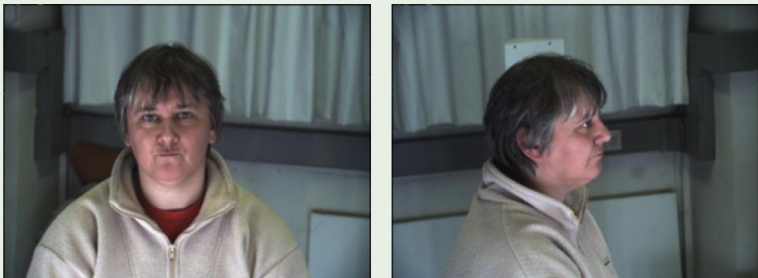

Task group: dynamic rotation (object)

Task: object\_rotation\_classification\_imagefirst

Question:

<image>  
<image>  
From a stationary viewpoint, in which direction did the object rotate between these two views? A. counterclockwise B. clockwise  
Only answer with the capital letter from (A, B).  
The camera is stationary and the object rotate in place.  
Clockwise and counterclockwise are defined from a top-down view.

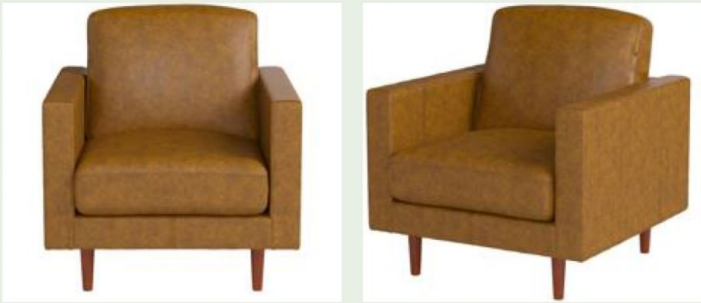

Task: object\_rotation\_classification\_interleaved

Question:

Looking at the object from a fixed camera position: <image>  
<image>  
Which rotation direction does the object show? A. clockwise B. counterclockwise  
Only answer with the capital letter from (A, B).  
The camera is stationary and the object rotate in place.  
Clockwise and counterclockwise are defined from a top-down view.

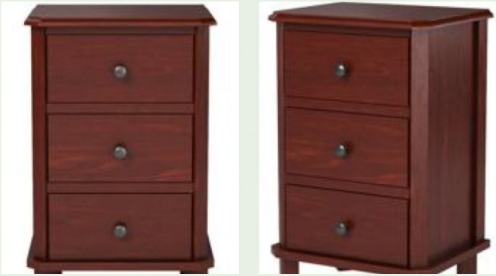

Task: object\_rotation\_classification\_textfirst

Question:

The viewpoint is static. Which way did the object turn — clockwise or counterclockwise? <image>  
<image>  
A. counterclockwise, B. clockwise  
Only answer with the capital letter from (A, B).  
The camera is stationary and the object rotate in place.  
Clockwise and counterclockwise are defined from a top-down view.

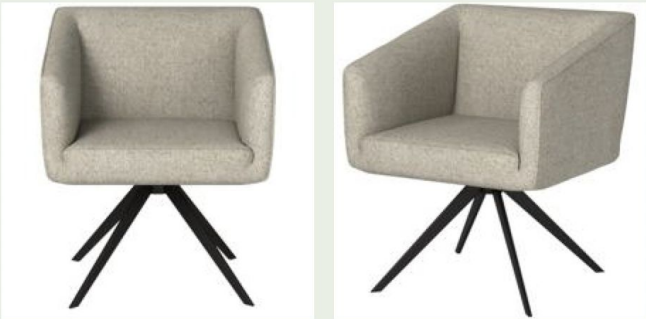



Task group: dynamic translation

Task: infinigen\_spatial\_relationship\_dynamic\_front\_back

Question:

From a static viewer's perspective, which direction did the pudding box change position from the first image <image> to the second image <image>?

- ☒ A. front ☐ B. back

Only answer with a single capital letter from (A, B).

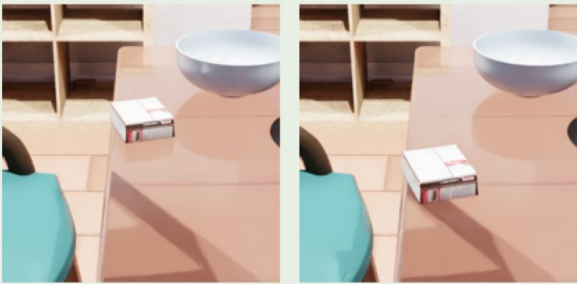

Task: infinigen\_spatial\_relationship\_dynamic\_front\_back

Question:

From a static viewer's perspective, which direction did the potted meat can change position from the first image <image> to the second image <image>?

- A. front ☐ B. back ☒

Only answer with a single capital letter from (A, B).

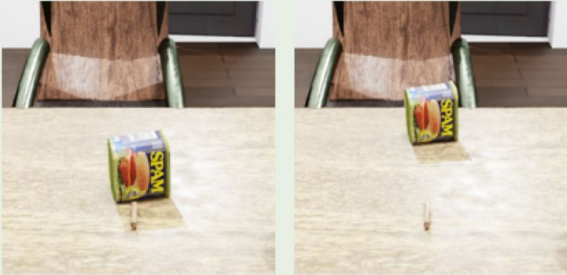

Task: infinigen\_spatial\_relationship\_dynamic\_left\_right

Question:

From a static viewer's perspective, which direction did the bleach cleanser change position from the first image <image> to the second image <image>?

- ☒ A. left ☐ B. right

Only answer with a single capital letter from (A, B).

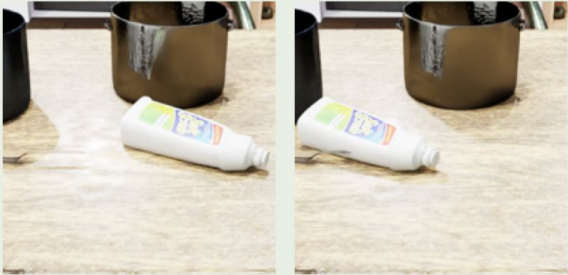

Task: infinigen\_spatial\_relationship\_dynamic\_left\_right

Question:

From a static viewer's perspective, which direction did the scissors change position from the first image <image> to the second image <image>?

- A. left ☐ B. right ☒

Only answer with a single capital letter from (A, B).

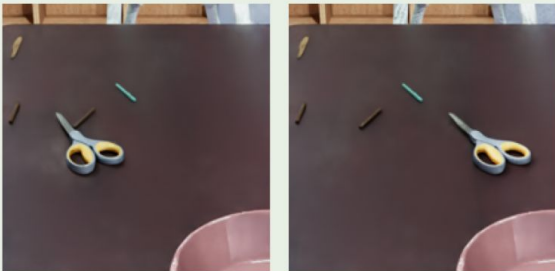



Task group: canonical view selection (car)

Task: car\_canonical\_view\_selection\_back

Question:

You are shown four images of a car in order: [1] Front view, [2] View A, [3] View B, [4] View C.  
Select the image that best shows the car from the back side.

Front view: <image>

A: <image>

B: <image>

C: <image>

Only answer with a single capital letter (A, B, or C).

The back side is defined from the viewer's perspective when looking at the front of the car.

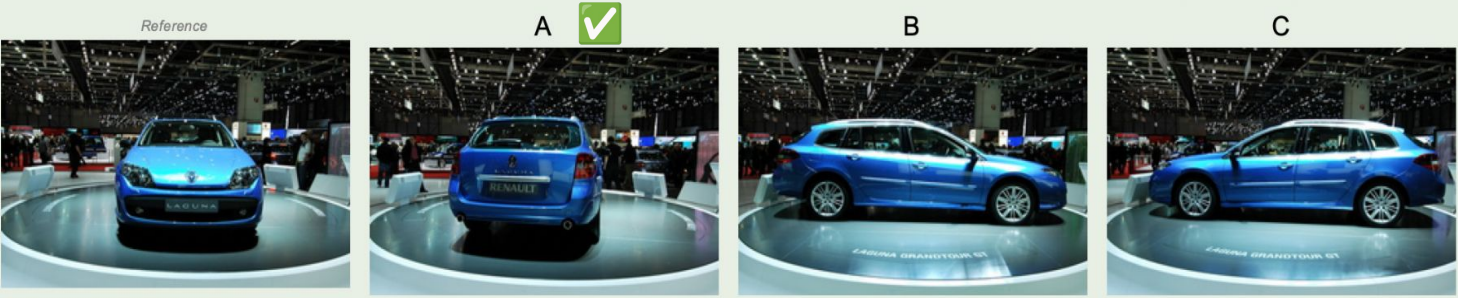

Task: car\_canonical\_view\_selection\_left

Question:

You are shown four images of a car in order: [1] Front view, [2] View A, [3] View B, [4] View C.  
Select the image that best shows the car from the left side.

Front view: <image>

A: <image>

B: <image>

C: <image>

Only answer with a single capital letter (A, B, or C).

The left side is defined from the viewer's perspective when looking at the front of the car.

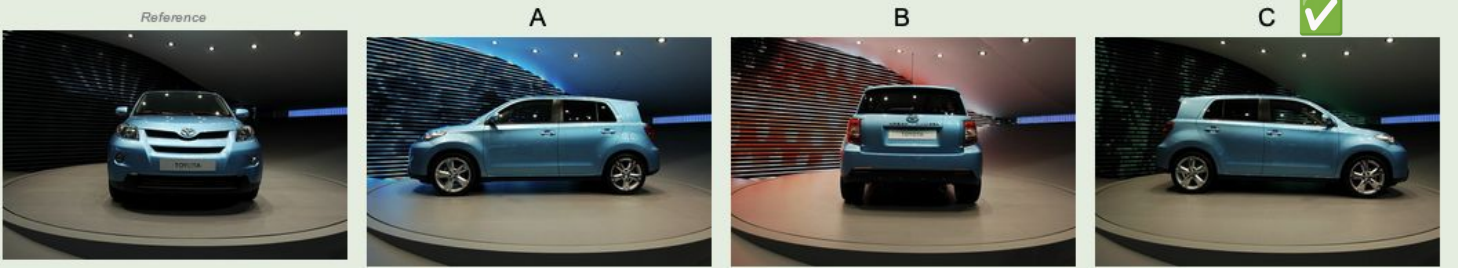

Task: car\_canonical\_view\_selection\_right

Question:

You are shown four images of a car in order: [1] Front view, [2] View A, [3] View B, [4] View C.  
Select the image that best shows the car from the right side.

Front view: <image>

A: <image>

B: <image>

C: <image>

Only answer with a single capital letter (A, B, or C).

The right side is defined from the viewer's perspective when looking at the front of the car.

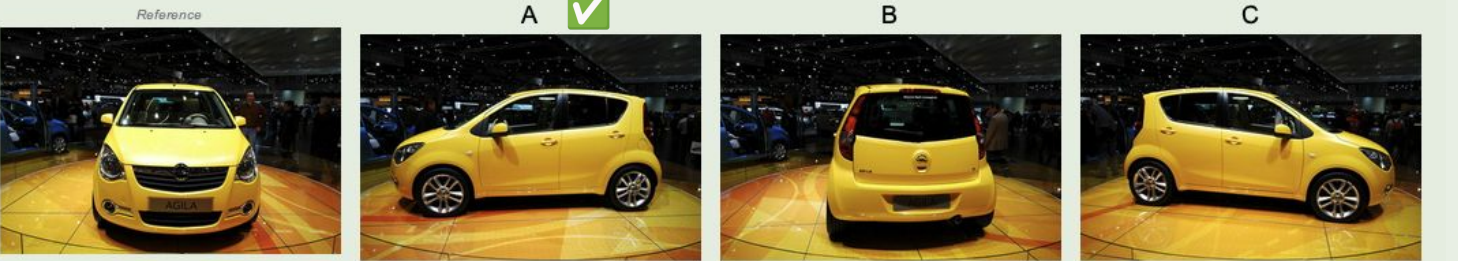



Task group: canonical view selection (face)

Task: face\_canonical\_view\_selection\_own\_perspective\_left

Question:

You are shown three images in order: [1] Front view, [2] View A, [3] View B.  
Select the image that best shows the left profile (person's own left).

Front view: <image>

A: <image>

B: <image>

Only answer with a single capital letter (A or B).

The left/right profile is defined from the person's own perspective (their left vs their right).

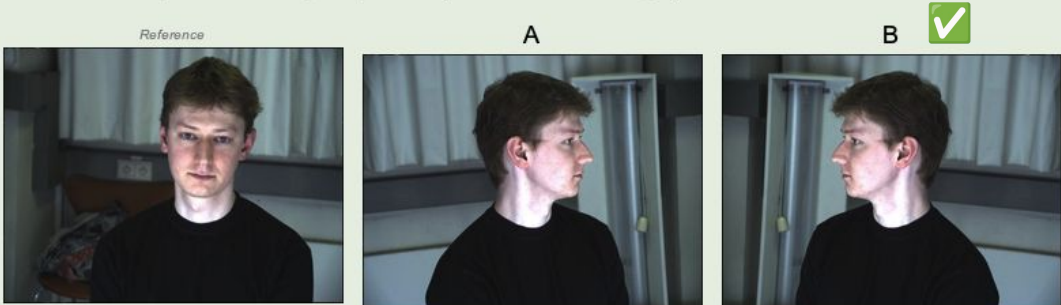

Task: face\_canonical\_view\_selection\_own\_perspective\_right

Question:

You are shown three images in order: [1] Front view, [2] View A, [3] View B.  
Select the image that best shows the right profile (person's own right).

Front view: <image>

A: <image>

B: <image>

Only answer with a single capital letter (A or B).

The left/right profile is defined from the person's own perspective (their left vs their right).

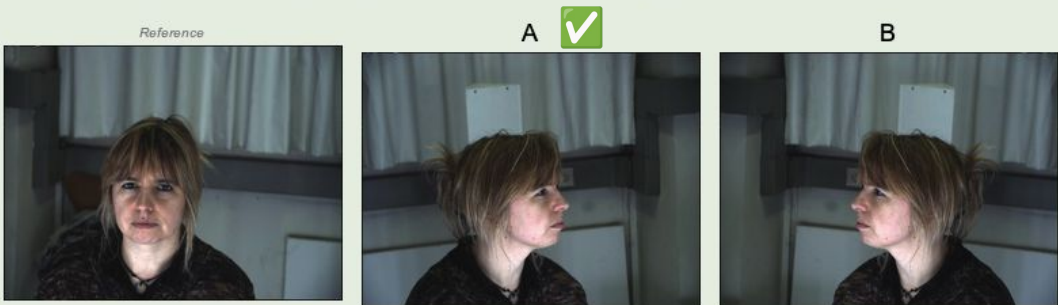

Task: face\_canonical\_view\_selection\_viewer\_perspective\_left

Question:

You are shown three images in order: [1] Front view, [2] View A, [3] View B.  
Select the image that best shows the left profile (viewer's left).

Front view: <image>

A: <image>

B: <image>

Only answer with a single capital letter (A or B).

The left/right profile is defined from your perspective as the viewer (your left vs your right when looking at the person).

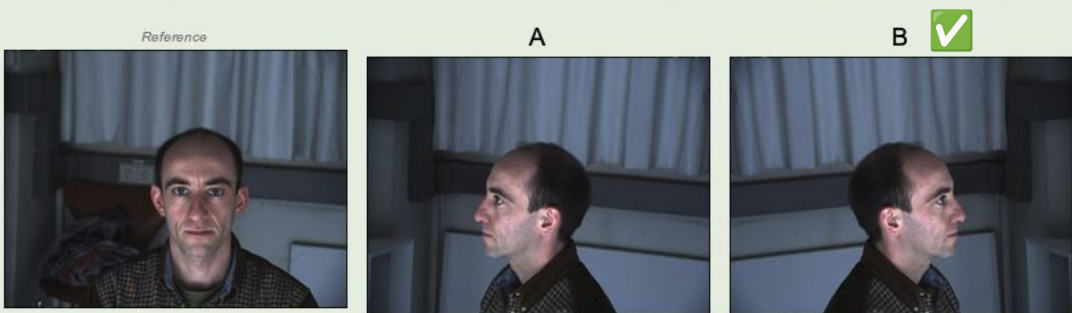

Task: face\_canonical\_view\_selection\_viewer\_perspective\_right

Question:

You are shown three images in order: [1] Front view, [2] View A, [3] View B.  
Select the image that best shows the right profile (viewer's right).

Front view: <image>

A: <image>

B: <image>

Only answer with a single capital letter (A or B).

The left/right profile is defined from your perspective as the viewer (your left vs your right when looking at the person).

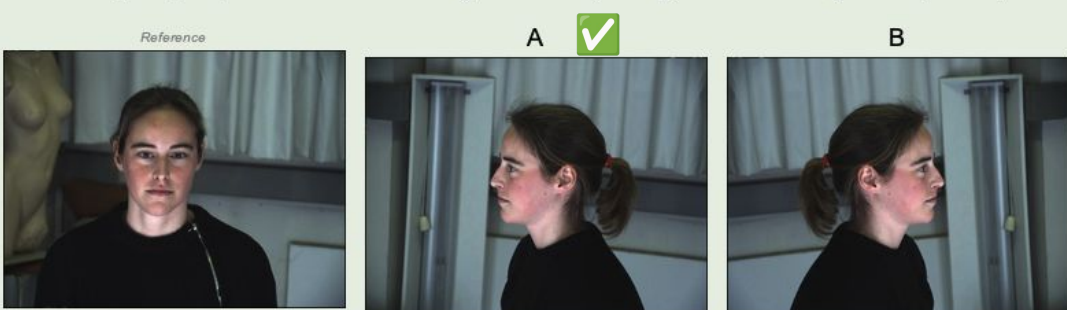



Task group: canonical view selection (object)

Task: object\_canonical\_view\_selection\_back

Question:

You are shown four images in order: [1] Front view, [2] View A, [3] View B, [4] View C.  
Select the image that best shows the object from the back side.  
Front view: <image>  
A: <image>  
B: <image>  
C: <image>Only answer with a single capital letter (A, B, or C).  
The back side is defined from the camera/viewer's perspective: 'back side' means the side that appears on the back when looking at the object from the front view.

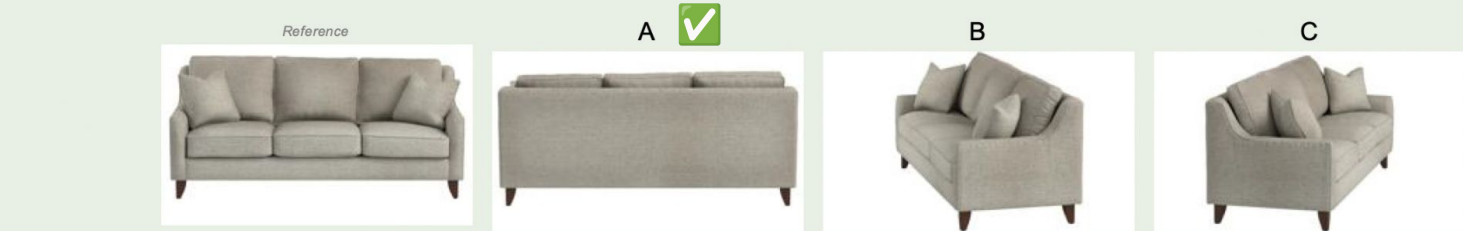

Task: object\_canonical\_view\_selection\_left

Question:

You are shown four images in order: [1] Front view, [2] View A, [3] View B, [4] View C.  
Select the image that best shows the object from the left side.  
Front view: <image>  
A: <image>  
B: <image>  
C: <image>Only answer with a single capital letter (A, B, or C).  
The left side is defined from the camera/viewer's perspective: 'left side' means the side that appears on the left when looking at the object from the front view.

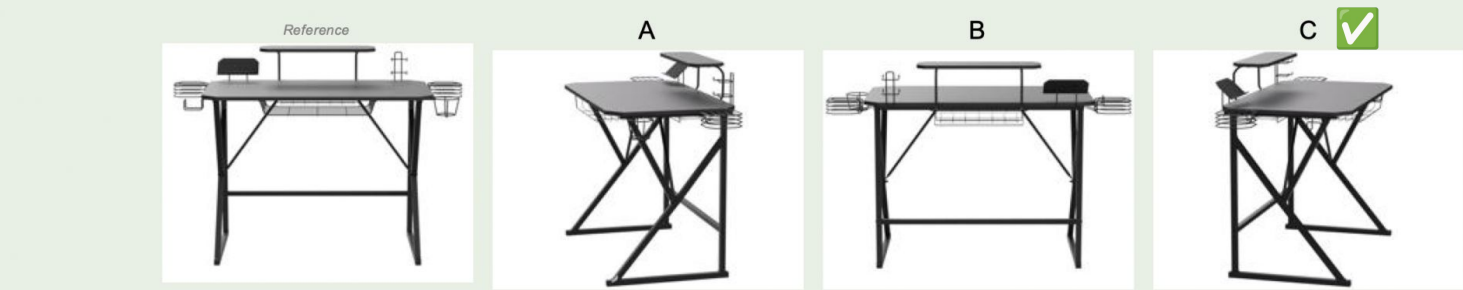

Task: object\_canonical\_view\_selection\_right

Question:

You are shown four images in order: [1] Front view, [2] View A, [3] View B, [4] View C.  
Select the image that best shows the object from the right side.  
Front view: <image>  
A: <image>  
B: <image>  
C: <image>Only answer with a single capital letter (A, B, or C).  
The right side is defined from the camera/viewer's perspective: 'right side' means the side that appears on the right when looking at the object from the front view.

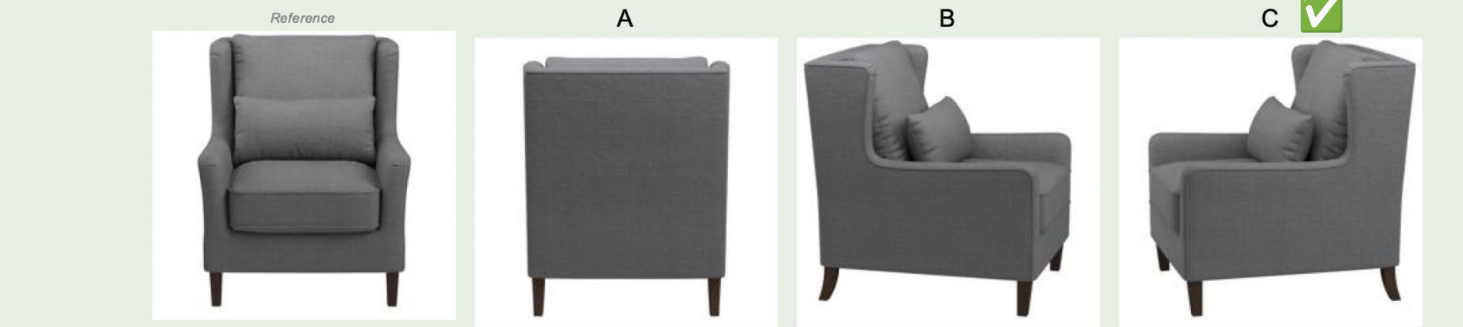

Task group: perspective taking (view selection + full occlusion)

Task: infinigen\_rotation\_selection\_back\_full\_occlusion

Question:

You are shown four images in order: [1] Front reference view containing the large marker, [2] View A, [3] View B, [4] View C. Views A, B, and C show the same scene from three distinct angles, left, right, and back in random order. From the viewer's perspective in the reference image.

<image>

Which of the three candidate views (A <image>, B <image>, or C <image>) is most likely taken from the back side of the large marker?

Only answer with a single capital letter from (A, B, C).

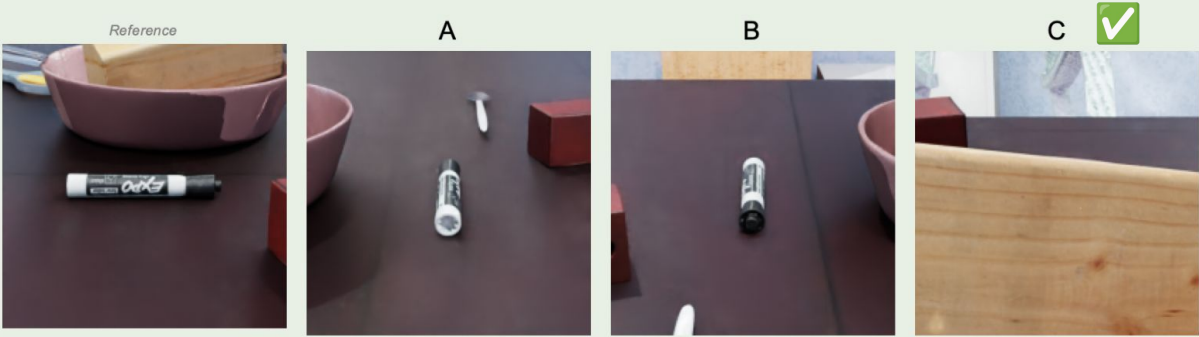

Task: infinigen\_rotation\_selection\_left\_full\_occlusion

Question:

You are shown four images in order: [1] Front reference view containing the gelatin box, [2] View A, [3] View B, [4] View C. Views A, B, and C show the same scene from three distinct angles, left, right, and back in random order. From the viewer's perspective in the reference image.

<image>

Which of the three candidate views (A <image>, B <image>, or C <image>) is most likely taken from the left side of the gelatin box?

Only answer with a single capital letter from (A, B, C).

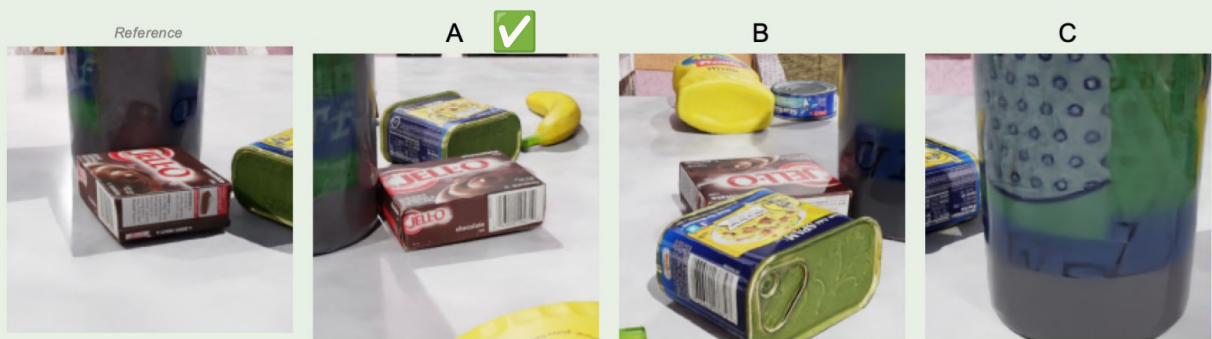

Task: infinigen\_rotation\_selection\_right\_full\_occlusion

Question:

You are shown four images in order: [1] Front reference view containing the bowl, [2] View A, [3] View B, [4] View C. Views A, B, and C show the same scene from three distinct angles, left, right, and back in random order. From the viewer's perspective in the reference image.

<image>

Which of the three candidate views (A <image>, B <image>, or C <image>) is most likely taken from the right side of the bowl?

Only answer with a single capital letter from (A, B, C).

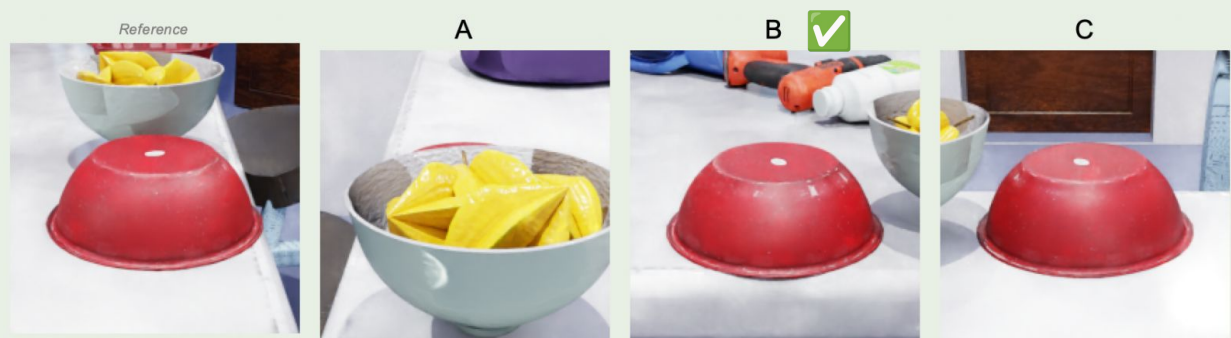



Task group: perspective taking (view selection + no occlusion)

Task: infinigen\_rotation\_selection\_back\_no\_occlusion

Question:

You are shown four images in order: [1] Front reference view containing the gelatin box, [2] View A, [3] View B, [4] View C. Views A, B, and C show the same scene from three distinct angles, left, right, and back in random order. From the viewer's perspective in the reference image. <image> Which of the three candidate views (A <image>, B <image>, or C <image>) is most likely taken from the back side of the gelatin box? Only answer with a single capital letter from (A, B, C).

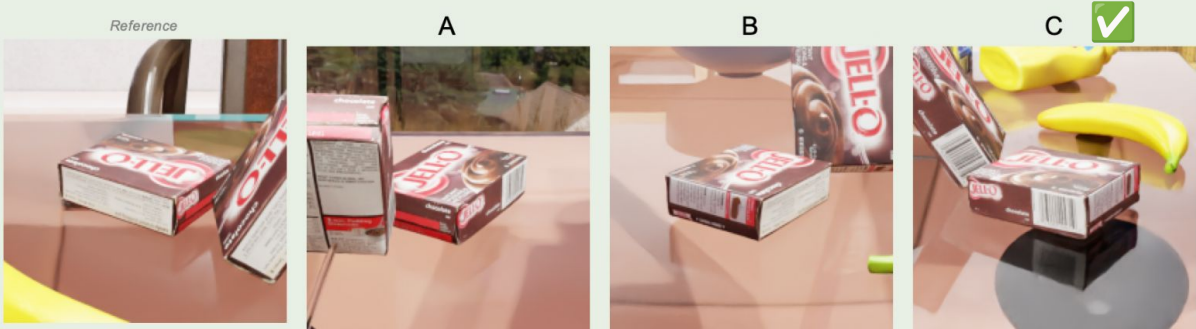

Task: infinigen\_rotation\_selection\_left\_no\_occlusion

Question:

You are shown four images in order: [1] Front reference view containing the large marker, [2] View A, [3] View B, [4] View C. Views A, B, and C show the same scene from three distinct angles, left, right, and back in random order. From the viewer's perspective in the reference image. <image> Which of the three candidate views (A <image>, B <image>, or C <image>) is most likely taken from the left side of the large marker? Only answer with a single capital letter from (A, B, C).

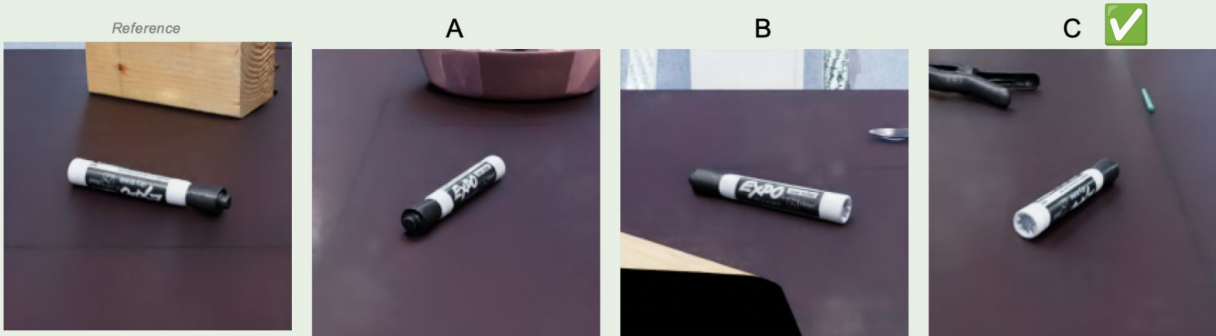

Task: infinigen\_rotation\_selection\_right\_no\_occlusion

Question:

You are shown four images in order: [1] Front reference view containing the banana, [2] View A, [3] View B, [4] View C. Views A, B, and C show the same scene from three distinct angles, left, right, and back in random order. From the viewer's perspective in the reference image. <image> Which of the three candidate views (A <image>, B <image>, or C <image>) is most likely taken from the right side of the banana? Only answer with a single capital letter from (A, B, C).

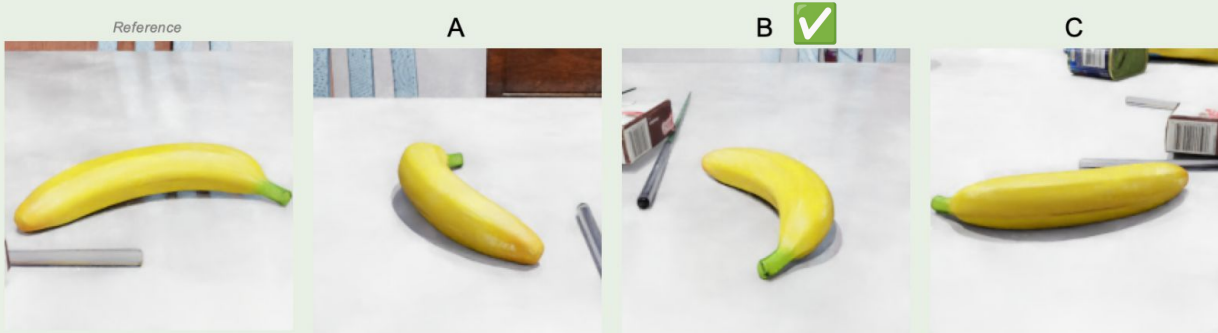

Task group: perspective taking (view selection + partial occlusion)

Task: infinigen\_rotation\_selection\_back\_partial\_occlusion

Question:

You are shown four images in order: [1] Front reference view containing the power drill, [2] View A, [3] View B, [4] View C. Views A, B, and C show the same scene from three distinct angles, left, right, and back in random order. From the viewer's perspective in the reference image.  
<image>  
Which of the three candidate views (A <image>, B <image>, or C <image>) is most likely taken from the back side of the power drill?  
Only answer with a single capital letter from (A, B, C).

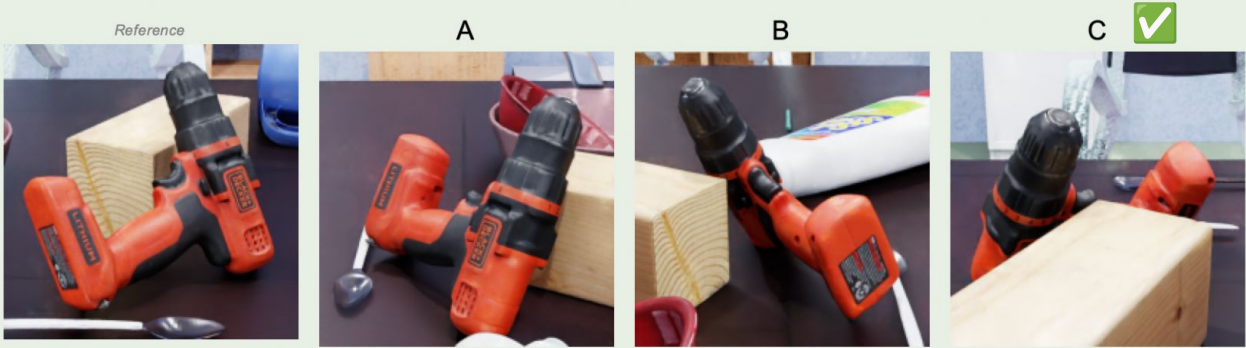

Task: infinigen\_rotation\_selection\_left\_partial\_occlusion

Question:

You are shown four images in order: [1] Front reference view containing the banana, [2] View A, [3] View B, [4] View C. Views A, B, and C show the same scene from three distinct angles, left, right, and back in random order. From the viewer's perspective in the reference image.  
<image>  
Which of the three candidate views (A <image>, B <image>, or C <image>) is most likely taken from the left side of the banana?  
Only answer with a single capital letter from (A, B, C).

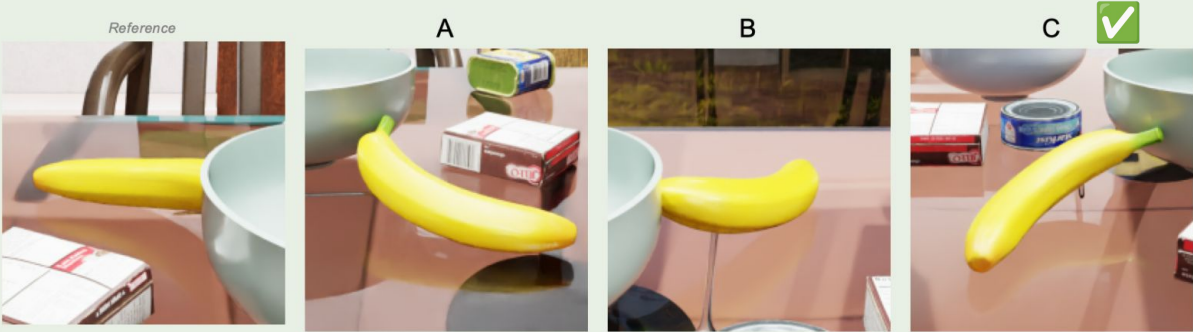

Task: infinigen\_rotation\_selection\_right\_partial\_occlusion

Question:

You are shown four images in order: [1] Front reference view containing the potted meat can, [2] View A, [3] View B, [4] View C. Views A, B, and C show the same scene from three distinct angles, left, right, and back in random order. From the viewer's perspective in the reference image.  
<image>  
Which of the three candidate views (A <image>, B <image>, or C <image>) is most likely taken from the right side of the potted meat can?  
Only answer with a single capital letter from (A, B, C).

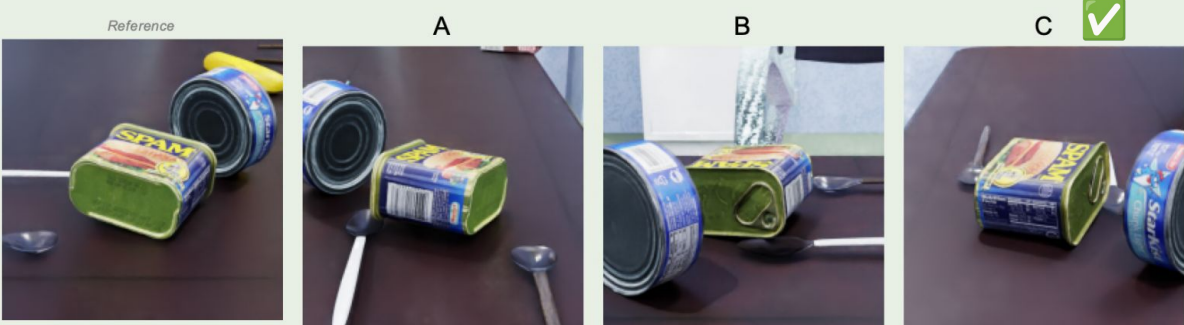



Task group: perspective taking (relative position transformation w/ premise)

Task: infinigen\_spatial\_relation\_transformation\_w\_premise\_back

Question:

<image>  
As pudding box is closer and potted meat can is farther from the viewer in the given front view, then when viewed from the back, which object is now closer to the viewer?  
A. potted meat can ☒  
B. pudding box  
Only answer with a single capital letter from (A, B).

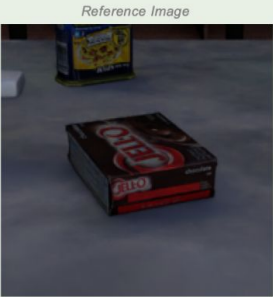

Task: infinigen\_spatial\_relation\_transformation\_w\_premise\_back

Question:

<image>  
As mustard bottle is on the left and mug is on the right in the given front view, then when viewed from the back, which object appears on the left from the new perspective?  
A. mustard bottle ☐  
B. mug ☒  
Only answer with a single capital letter from (A, B).

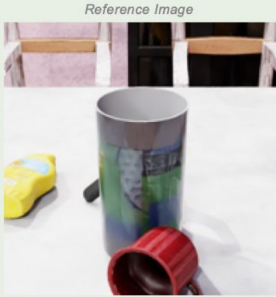

Task group: perspective taking (relative position transformation w/ premise)

Task: infinigen\_spatial\_relation\_transformation\_w\_premise\_left

Question:

<image>  
As potted meat can is closer and pudding box is farther from the viewer in the given front view, then when viewed from the viewer's left side, which object appears on the left from the new perspective?  
A. potted meat can  
B. pudding box ☒  
Only answer with a single capital letter from (A, B).

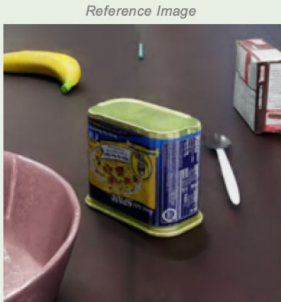

Task: infinigen\_spatial\_relation\_transformation\_w\_premise\_left

Question:

<image>  
As rubiks cube is on the left and mug is on the right in the given front view, then when viewed from the viewer's left side, which object is closer to the viewer?  
A. mug  
B. rubiks cube ☒  
Only answer with a single capital letter from (A, B).

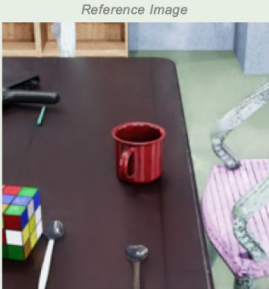



Task group: perspective taking (relative position transformation w/ premise)

Task: infinigen\_spatial\_relation\_transformation\_w\_premise\_right

Question:

<image>  
As large marker is closer and large clamp is farther from the viewer in the given front view, then when viewed from the viewer's right side, which object appears on the left from the new perspective?  
A. large marker ☒  
B. large clamp  
Only answer with a single capital letter from (A, B).

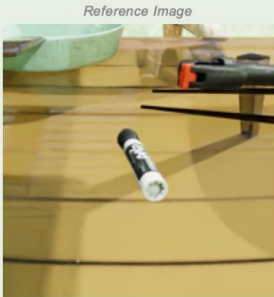

Task: infinigen\_spatial\_relation\_transformation\_w\_premise\_right

Question:

<image>  
As mug is on the left and rubiks cube is on the right in the given front view, then when viewed from the viewer's right side, which object is closer to the viewer?  
A. mug ☒  
B. rubiks cube  
Only answer with a single capital letter from (A, B).

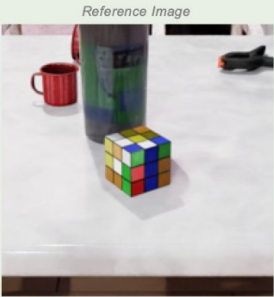

Task group: perspective taking (relative position transformation w/o premise)

Task: infinigen\_spatial\_relation\_transformation\_wo\_premise\_back

Question:

<image>  
The image shows the front view of a scene. Now imagine viewing the same scene from the back. From the new perspective, which object appears on the left?  
A. large marker ☒  
B. large clamp  
Only answer with a single capital letter from (A, B).

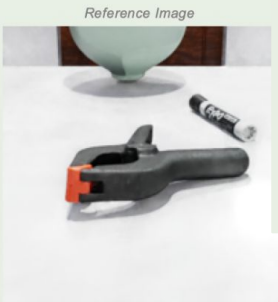

Task: infinigen\_spatial\_relation\_transformation\_wo\_premise\_back

Question:

<image>  
The image shows the front view of a scene. Now imagine viewing the same scene from the back. From the new perspective, which object is closer to the viewer?  
A. large marker ☒  
B. large clamp  
Only answer with a single capital letter from (A, B).

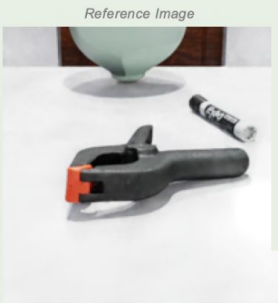



## Task group: perspective taking (relative position transformation w/o premise)

### Task: infinigen\_spatial\_relation\_transformation\_wo\_premise\_left

Question:

<image>  
The image shows the front view of a scene. Now imagine viewing the same scene from the viewer's left side. From the new perspective, which object is closer to the viewer?  
A. pitcher base  
B. mustard bottle ☒  
Only answer with a single capital letter from (A, B).

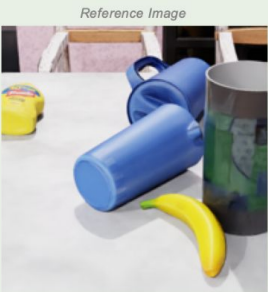

### Task: infinigen\_spatial\_relation\_transformation\_wo\_premise\_left

Question:

<image>  
The image shows the front view of a scene. Now imagine viewing the same scene from the viewer's left side. From the new perspective, which object now appears on the left?  
A. potted meat can  
B. pudding box ☒  
Only answer with a single capital letter from (A, B).

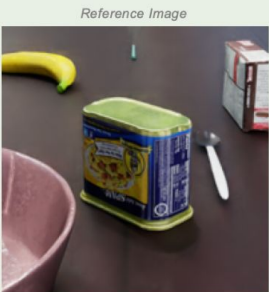

Task group: perspective taking (relative position transformation w/o premise)

Task: infinigen\_spatial\_relation\_transformation\_wo\_premise\_right

Question:

<image>  
The image shows the front view of a scene. Now imagine viewing the same scene from the viewer's right side. From the new perspective, which object is closer to the viewer?  
A. tuna fish can ☒  
B. pudding box  
Only answer with a single capital letter from (A, B).

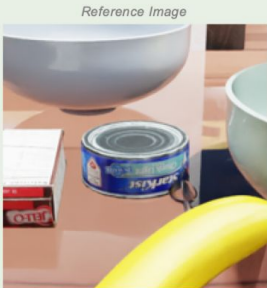

Task: infinigen\_spatial\_relation\_transformation\_wo\_premise\_right

Question:

<image>  
The image shows the front view of a scene. Now imagine viewing the same scene from the viewer's right side. From the new perspective, which object now appears on the left?  
A. master chef can  
B. sugar box ☒  
Only answer with a single capital letter from (A, B).

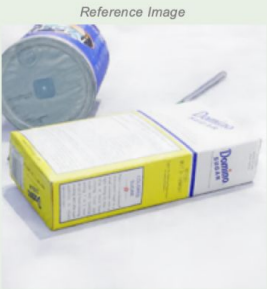



Task group: static object-relation grounding (left/right)

Task: infinigen\_spatial\_relation\_grounding\_left\_right

Question:

<image>  
From the viewer's perspective, is rubiks cube on the left or right of mustard bottle in the image?  
A. left, B. right ☒ ☐  
Only answer with a single capital letter from (A, B).

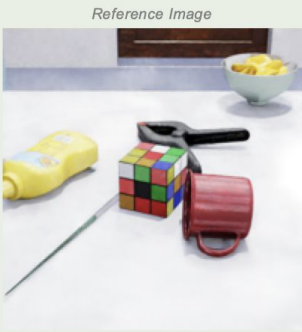

Symmetrical Augmentation:

Question:

<image>  
From the viewer's perspective, is mustard bottle on the left or right of rubiks cube in the image?  
☒ A. left, B. right ☐  
Only answer with a single capital letter from (A, B).

Syntactic Augmentation:

Question:

<image>  
From the viewer's perspective, which object is on the left in the image?  
☒ A. mustard bottle B. rubiks cube ☐  
Only answer with a single capital letter from (A, B).

Question:

<image>  
From the viewer's perspective, which object is on the right in the image?  
A. mustard bottle B. rubiks cube ☒ ☐  
Only answer with a single capital letter from (A, B).

Task group: static object-relation grounding (far/near)

Task: infinigen\_spatial\_relation\_grounding\_far\_near

Question:

<image>

Which object is closer to the viewer in the image?

☒ A. large marker, B.foam brick

Only answer with a single capital letter from (A, B).

Reference Image

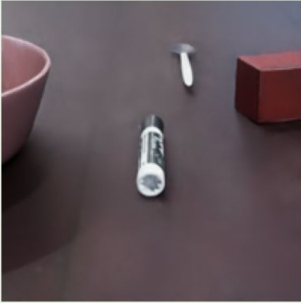

Symmetrical Augmentation:

Question:

<image>

Which object is farther from the viewer in the image?

A. large marker, B.foam brick ☒

Only answer with a single capital letter from (A, B).



Task group: static object-relation grounding (front/behind)

Task: infinigen\_spatial\_relationship\_front\_behind

Question:

<image>  
The image is taken from the front of the scene. Which object is in the front?  
☒ A. mug ☐ B.rubiks cube  
Only answer with a single capital letter from (A, B).

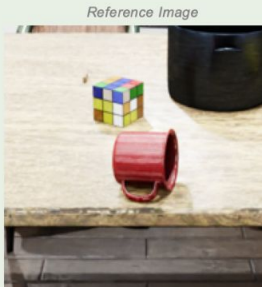

Symmetrical Augmentation:

Question:

<image>  
The image is taken from the front of the scene. Which object is in the back?  
A. mug, ☒ B.rubiks cube ☒  
Only answer with a single capital letter from (A, B).

Syntactic Augmentation:

Question:

<image>  
The image is taken from the front of the scene. Is mug positioned in front of rubiks cube or behind?  
☒ A. in front of ☐ B. behind  
Only answer with a single capital letter from (A, B).

Question:

<image>  
The image is taken from the front of the scene. Is rubiks cube positioned in front of mug or behind?  
A. in front of ☐ B. behind ☒  
Only answer with a single capital letter from (A, B).

Task group: mental rotation

Task: object\_mental\_rotation

Question:

<image>  
From the original viewpoint, the object spins 135 degrees clockwise. Which view shows the new orientation?  
A. <image>  
B. <image>  
C. <image>  
D. <image>  
Only answer with the captial letter from (A, B, C, D).

Reference Image

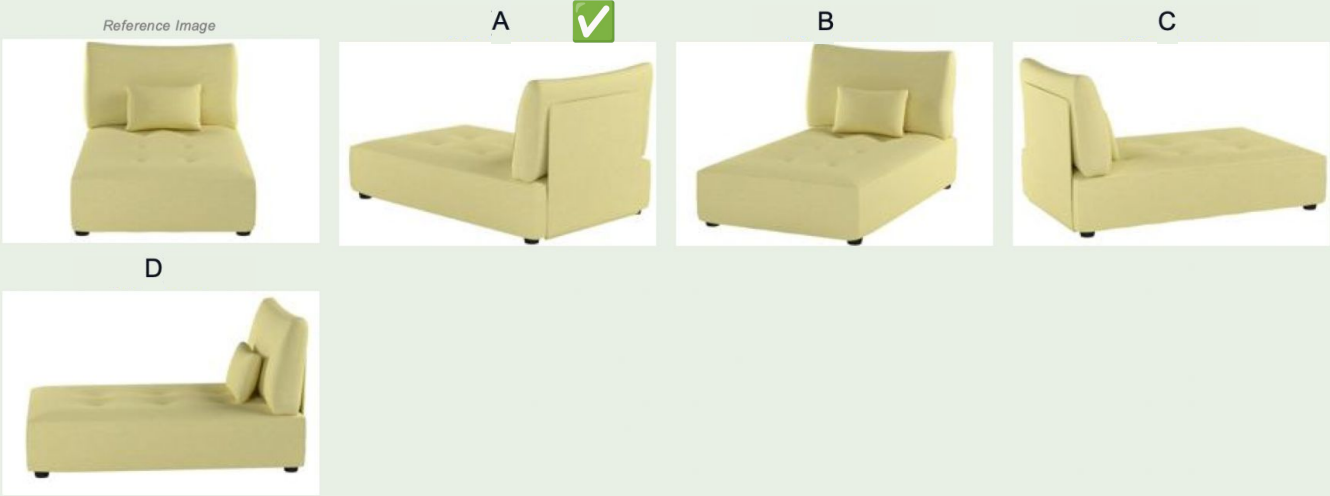

D

A

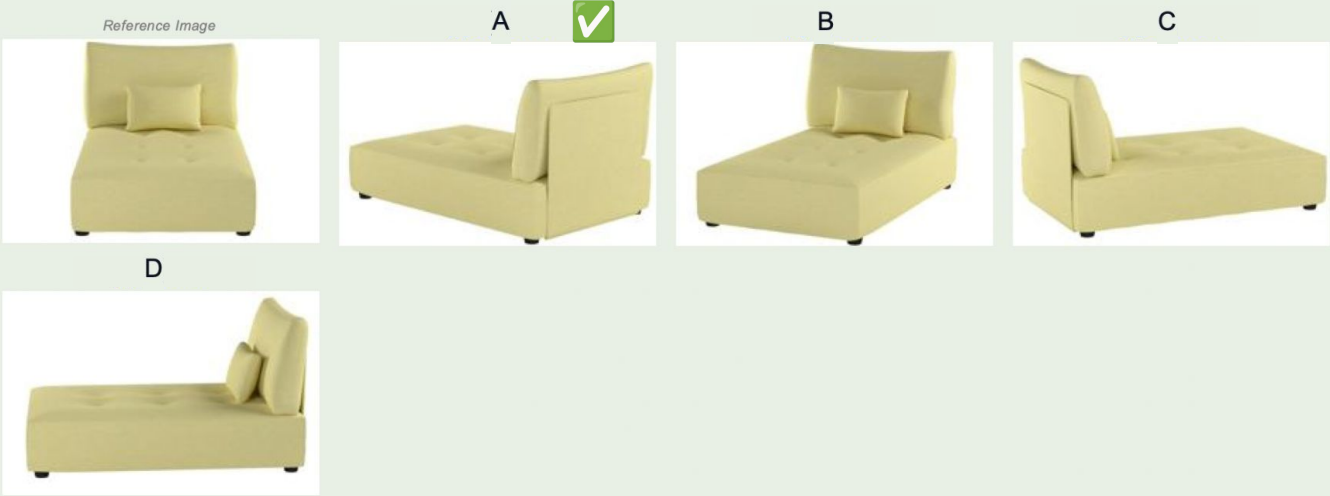

☒

B

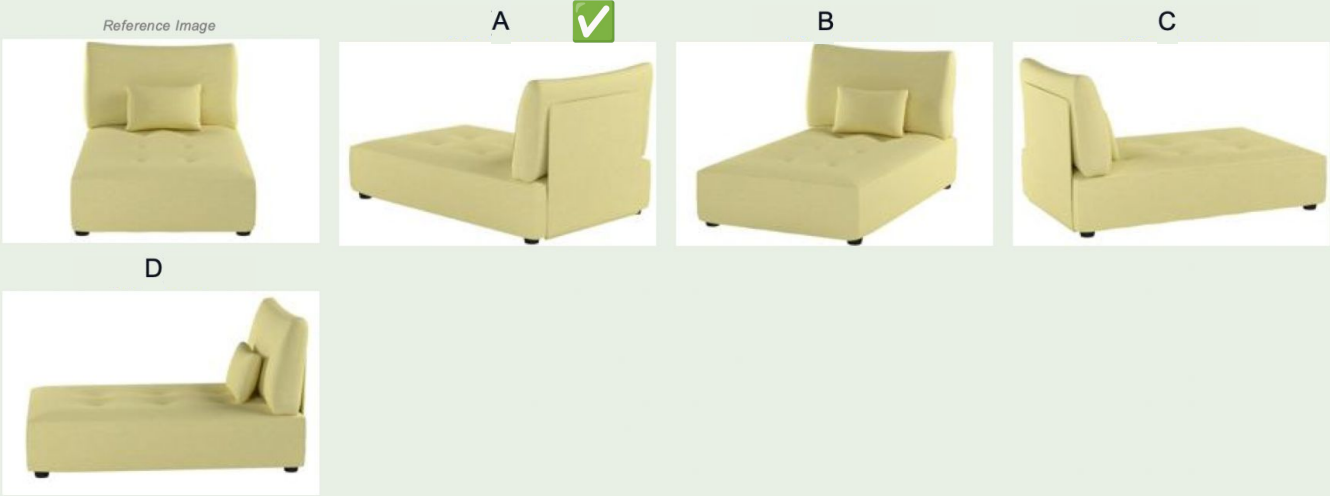

C

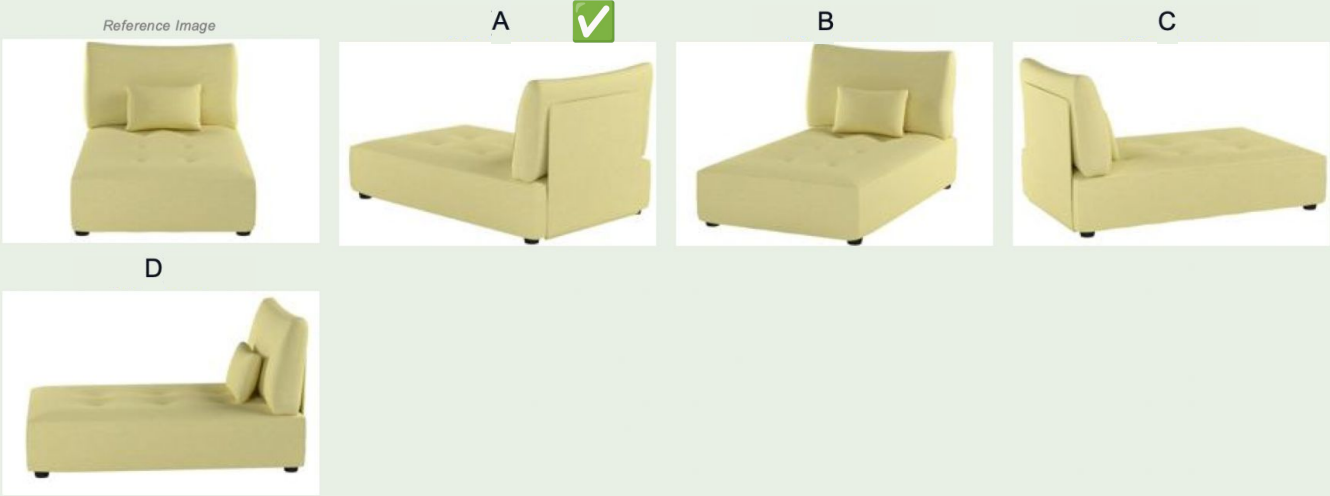



### Identity matching

- Which of these four images (A, B, C, D) shows a different car from the other three?

Quartet 3+1

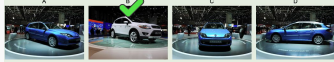

- Which of these three images (A, B, C) shows a different car from the other two?

Triplet 2+1

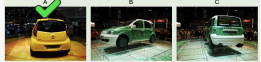

### Dynamic rotation

- Which way did the object turn? Clockwise is defined relative to a top-down view, with the object rotating in place.

A. clockwise, B. counterclockwise

- From the **person's own** perspective, which way did they turn?

A. right, B. left

- From the **viewer's** perspective, which way did the person turn?

A. right, B. left

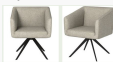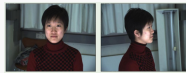

### Dynamic translation

- Which direction did the scissors change position from the first image to the second image?

A. left, B. right

- Which direction did the pudding box change position from the first image to the second image?

A. front, B. back

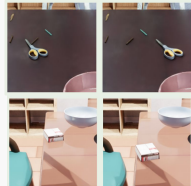

### Object-relation grounding

Symmetrical Augmentation

Syntactic Augmentation

- Which object is in the **front**? A. mug, B. rubik's cube
- Which object is in the **back**? A. mug, B. rubik's cube

- Is the **mug** in front of the **rubik's cube** or behind? A. in front of, B. behind

- Is the **rubik's cube** in front of the **mug** or behind? A. in front of, B. behind

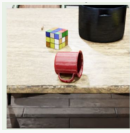

Seed Question

- Is **rubik's cube** on the left or right of the **mustard bottle**? A. left, B. right

- Is **mustard bottle** on the left or right of the **rubik's cube**? A. left, B. right

- Which object is on the **left**?

A. mustard bottle, B. rubik's cube

- Which object is on the **right**?

A. mustard bottle, B. rubik's cube

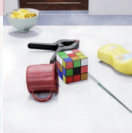

- Which object is **closer** to the viewer in the image?

A. large marker, B. foam brick

- Which object is **farther** from the viewer in the image?

A. large marker, B. foam brick

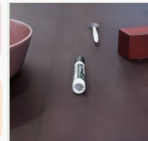

### Mental rotation

- The object spins 135 degrees clockwise. Which view from the four images (A, B, C, D) shows the new orientation?

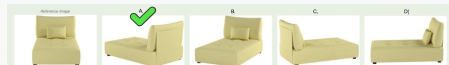

### Canonical view selection

- Select the image that best shows the object from the **left** side. Left side is defined from the viewer's perspective.

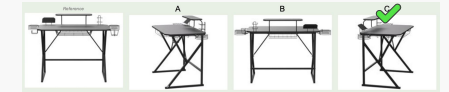

### Perspective taking

Scene Selection (S)

- Given front reference view, which of the three candidate views (A, B, C) is most likely taken from the **left**?

Partial occlusion

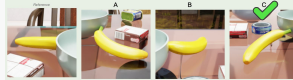

- Given front reference view, which of the three candidate views (A, B, C) is most likely taken from the **back**?

No occlusion

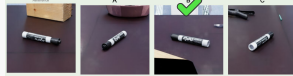

Relation Transformation (T)

When viewing from the **back**:

- which object appears closer to viewer?

A. clamp B. marker

When viewing from the **left**:

- which object appears on the left?

A. meat can, B. pudding box

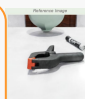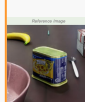

Relation Transformation (T) with premise

As the **clamp is in the front** and **marker is in the back** in the front view, when viewing from the **back**:

- which object appears closer to viewer?

A. clamp B. marker

As the **meat can is closer** and **pudding box is farther** from the **viewer** in the front view, when viewing from the **left**:

- which object appears on the left?

A. meat can, B. pudding box

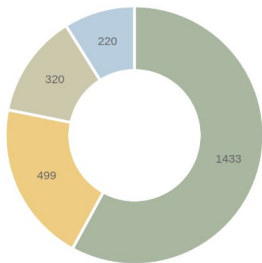

Task Groups

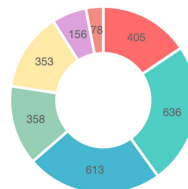

- Identity Matching (15.6%)
- Perspective Taking (23.6%)
- Canonical View Selection (13.8%)
- Dynamic Rotation (13.6%)
- Dynamic Translation (6.0%)
- Mental Rotation (3.0%)
- Static Inter-Object (24.5%)
